# Supplementary material for: Automated Verification of Silq Quantum Programs using SMT Solvers
Source: arXiv:2406.03119 source file (2024-06-05)
Supplement: Supplementary file 1 [file appendix.tex]

\section{Quantum Computing Basics}
\label{sec:basicqc}
\input{Sections/qc}
%\section{Example Algorithms}
%\input{Sections/examples}
